# Supplementary material for: An Introduction to Permutation Processes (version 0.5)
Source: arXiv:2407.09664 source file (2024-07-12)
Supplement: Supplementary file 1 [file appendix.tex]

\begin{partbacktext}
\part{Appendices}
\end{partbacktext}

\appendix

\chapter{Collections}
\label{appendix:collections}

\abstract{This appendix gives a description of the vector collections used in experiments
throughout this monograph. These collections demonstrate different operating points in
a typical use-case. For example, some consist of dense vectors, others of sparse vectors;
some have few dimensions and others are in much higher dimensions; some are relatively small
while others contain a large number of points.}

\bigskip

Table~\ref{table:appendix:collections:dense} gives a description of the dense vector collections
used throughout this monograph and summarizes their key statistics.

\begin{table*}[ht]
\caption{Dense collections used in this monograph along with select statistics.}
\scriptsize
\label{table:appendix:collections:dense}
\begin{center}
\begin{sc}
\begin{tabular}{p{5cm}|ccc}
\toprule
Collection & Vector Count & Query Count & Dimensions \\
\midrule
\textsc{GloVe}-$25$~\citep{pennington-etal-2014-glove} & $1.18$M & $10{,}000$ & $25$ \\
\textsc{GloVe}-$50$ & $1.18$M & $10{,}000$ & $50$ \\
\textsc{GloVe}-$100$ & $1.18$M & $10{,}000$ & $100$ \\
\textsc{GloVe}-$200$ & $1.18$M & $10{,}000$ & $200$ \\
\textsc{Deep1b}~\citep{deep1b} & $9.99$M & $10{,}000$ & $96$ \\
\textsc{MS Turing}~\citep{msturingDataset} & $10$M & $100{,}000$ & $100$ \\
\textsc{Sift}~\citep{Lowe2004DistinctiveIF} & $1$M & $10{,}000$ & $128$ \\
\textsc{Gist}~\citep{Oliva2001ModelingTS} & $1$M & $1{,}000$ & $960$ \\
\bottomrule
\end{tabular}
\end{sc}
\end{center}
\end{table*}

In addition to the vector collections above, we convert a few text collections
into vectors using various embedding models. These collections are described in
Table~\ref{table:appendix:collections:text}. Please see~\citep{nguyen2016msmarco} for
a complete description of the MS MARCO v1 collection and~\citep{thakur2021beir} for the others.

\begin{table*}[ht]
\caption{Text collections along with key statistics.
The rightmost two columns report the average number of non-zero
entries in data points and, in parentheses, queries for sparse vector
representations of the collections.}
\scriptsize
\label{table:appendix:collections:text}
\begin{center}
\begin{sc}
\begin{tabular}{c|cc|cc}
\toprule
Collection & Vector Count & Query Count & \splade{} & \esplade{}\\
\midrule
\textsc{MS Marco} Passage& $8.8$M & $6{,}980$ & 127 (49) & 185 (5.9) \\
NQ & $2.68$M & $3{,}452$ & 153 (51) & 212 (8) \\
\textsc{Quora} & $523$K & $10{,}000$ & 68 (65) & 68 (8.9) \\
\textsc{HotpotQA} & $5.23$M & $7{,}405$ & 131 (59) & 125 (13) \\
\textsc{Fever} & $5.42$M & $6{,}666$ & 145 (67) & 140 (8.6) \\
\textsc{DBPedia} & $4.63$M & $400$ & 134 (49) & 131 (5.9) \\
\bottomrule
\end{tabular}
\end{sc}
\end{center}
\end{table*}

When transforming the text collections of Table~\ref{table:appendix:collections:text}
into vectors, we use the following embedding models:
\begin{itemize}
    \item \textsc{AllMiniLM-l6-v2}:\footnote{Available at \url{https://huggingface.co/sentence-transformers/all-MiniLM-L6-v2}}
    Projects text documents into $384$-dimensional dense vectors for retrieval with angular distance.

    \item \textsc{Tas-B}~\citep{tas-b}: A bi-encoder model that was trained using supervision from a cross-encoder and a ColBERT~\citep{colbert2020khattab} model,
    and produces $768$-dimensional dense vectors that are meant for MIPS.
    The checkpoint used in this work is available on HuggingFace.\footnote{Available at \url{https://huggingface.co/sentence-transformers/msmarco-distilbert-base-tas-b}}

    \item \splade{}~\citep{formal2022splade}:\footnote{Pre-trained checkpoint from HuggingFace available at \url{https://huggingface.co/naver/splade-cocondenser-ensembledistil}}
    Produces sparse representations for text.
    The vectors have roughly $30{,}000$ dimensions, where each dimension corresponds
    to a term in the BERT~\citep{devlin2019bert} WordPiece~\citep{wordpiece} vocabulary.
    Non-zero entries in a vector reflect learnt term importance weights.

    \item \esplade{}~\citep{lassance2022sigir}:\footnote{Pre-trained checkpoints for document and
    query encoders were obtained from \url{https://huggingface.co/naver/efficient-splade-V-large-doc} and \url{https://huggingface.co/naver/efficient-splade-V-large-query},
    respectively.}
    This model produces queries that have far fewer non-zero entries than the original
    \splade{} model, but documents that may have a larger number of non-zero entries.
\end{itemize}

\bibliographystyle{abbrvnat}
\bibliography{biblio}

\chapter{Probability Review}
\label{appendix:probability}

\abstract{We briefly review key concepts in probability in this appendix.}

\section{Probability}
We identify a \emph{probability space} denoted by $(\Omega, \mathcal{F}, \probability)$
with an \emph{outcome space}, an \emph{events} set, and a \emph{probability measure}.
The outcome space, $\Omega$, is the set of all
possible outcomes. For example, when flipping a two-sided coin, the outcome
space is simply $\{0, 1\}$. When rolling a six-sided die, it is instead
the set $[6] = \{ 1, 2, \ldots, 6\}$.

The events set $\mathcal{F}$ is a set of subsets of $\Omega$ that
includes $\Omega$ as a member and is closed under complementation and
countable unions. That is, if $E \in \mathcal{F}$,
then we must have that $E^\complement \mathcal{F}$.
Furthermore, the union of countably many events $E_i$'s
in $\mathcal{F}$ is itself in $\mathcal{F}$: $\cup_i E_i \in \mathcal{F}$.
A set $\mathcal{F}$ that satisfies these properties is called a $\sigma$-algebra.

Finally, a function $\probability: \mathcal{F} \rightarrow \mathbb{R}$ is
a probability measure if it satisfies the following conditions: $\probability[\Omega] = 1$;
$\probability[E] \geq 0$ for any event $E \in \mathcal{F}$;
$\probability[E^\complement] = 1 - \probability[E]$; and, finally,
for countably many disjoint events $E_i$'s:
$\probability[\cup_i E_i] = \sum_i \probability[E_i]$.

We should note that, $\probability$ is also known as a ``probability distribution''
or simply a ``distribution.'' The pair $(\Omega, \mathcal{F})$ is called
a \emph{measurable space}, and the elements of $\mathcal{F}$ are
known as a \emph{measurable sets}. The reason they are called ``measurable''
is because they can be ``measured'' with $\probability$: The function
$\probability$ assigns values to them.

In many of the discussions throughout this monograph, we omit the outcome space
and events set because that information is generally clear from context.
However, a more formal treatment of our arguments requires a complete
definition of the probability space.

\section{Random Variables}
A random variable on a measurable space $(\Omega, \mathcal{F})$ is
a measurable function $X: \Omega \rightarrow \mathbb{R}$.
It is measurable in the sense that the \emph{preimage} of any Borel set $B \in \mathcal{B}$
is an event: $X^{-1}(B) = \{ \omega \in \Omega \;|\; X(\omega) \in B \} \in \mathcal{F}$.

A random variable $X$ generates a $\sigma$-algebra that comprises of the preimage
of all Borel sets. It is denoted by $\sigma(X)$
and formally defined as $\sigma(X) = \{ X^{-1}(B) \;|\; B \in \mathcal{B} \}$.

\bigskip

Random variables are typically categorized as discrete or continuous.
$X$ is \emph{discrete} when it maps $\Omega$ to a discrete set.
In that case, its \emph{probability mass function} is defined as $\probability[X = x]$
for some $x$ in its range.
A \emph{continuous} random variable is often associated with a
probability \emph{density} function, $f_X$, such that:
\begin{equation*}
    \probability[a \leq X \leq b] = \int_a^b f_X(x) dx.
\end{equation*}

Consider, for instance, the following probability density function over the real line for
parameters $\mu \in \mathbb{R}$ and $\sigma > 0$:
\begin{equation*}
    f(x) = \frac{1}{\sqrt{2 \pi \sigma^2}} e^{- \frac{(x - \mu)^2}{2\sigma^2}}.
\end{equation*}
A random variable with the density function above is said to follow a Gaussian
distribution with mean $\mu$ and variance $\sigma^2$, denoted by $X \sim \mathcal{N}(\mu, \sigma^2)$.
When $\mu = 0$ and $\sigma^2 = 1$, the resulting distribution is called the standard
Normal distribution.

Gaussian random variables have attractive properties.
For example, the sum of two independent Gaussian random variables is itself a Gaussian variable.
Concretely, $X_1 \sim \mathcal{N}(\mu_1, \sigma_1^2)$ and $X_2 \sim \mathcal{N}(\mu_2, \sigma_2^2)$,
then $X_1 + X_2 \sim \mathcal{N}(\mu_1 + \mu_2, \sigma_1^2 + \sigma_2^2)$.
The sum of the squares of $m$ independent Gaussian random variables, on the other hand,
follows a $\chi^2$-distribution with $m$ degrees of freedom.

\section{Conditional Probability}
Conditional probabilities give us a way to model how the probability of an event changes
in the presence of extra information, such as partial knowledge about a random outcome.
Concretely, if $(\Omega, \mathcal{F}, \probability)$ is a probability space and
$A, B \in \mathcal{F}$ such that $\probability[B] > 0$, then the \emph{conditional
probability} of $A$ given the event $B$ is denoted by $\probability[A \;\lvert\; B]$ and
defined as follows:
\begin{equation*}
    \probability[A \;\lvert\; B] = \frac{\probability[A \cap B]}{\probability[B]}.
\end{equation*}

We use a number of helpful results concerning conditional probabilities
in proofs throughout the monograph. One particularly useful inequality
is what is known as the \emph{union bound} and is stated as follows:
\begin{equation*}
    \probability[\cup_i A_i] \leq \sum_i \probability[A_i].
\end{equation*}

Another fundamental property is the law of total probability.
It states that, for mutually disjoint events $A_i$'s such that
$\Omega = \cup A_i$, the probability of any event $B$ can be expanded
as follows:
\begin{equation*}
    \probability[B] = \sum_i \probability[B \;\lvert\; A_i] \probability[A_i].
\end{equation*}
This is easy to verify: the summand is by definition equal to $\probability[B \cap A_i]$
and, considering the events $(B \cap A_i)$'s are mutually disjoint, their sum
is equal to $\probability[B \cap (\cup A_i)] = \probability[B]$.

\section{Independence}
Another tool that reflects the effect (or lack thereof) of additional knowledge on probabilities
is the concept of \emph{independence}. Two events $A$ and $B$ are said to be
\emph{independent} if $\probability[A \cap B] = \probability[A] \times \probability[B]$.
Equivalently, we say that $A$ is independent of $B$ if and only if
$\probability[A \;\lvert\; B] = \probability[A]$ when $\probability[B] > 0$.

\bigskip

Independence between two random variables is defined similarly but requires a bit more care.
If $X$ and $Y$ are two random variables and $\sigma(X)$ and $\sigma(Y)$ denote
the $\sigma$-algebras generated by them, then $X$ is independent of $Y$ if
all events $A \in \sigma(X)$ and $B \in \sigma(Y)$ are independent.

When a sequence of random variables are \emph{mutually} independent and are drawn
from the same distribution (i.e., have the same probability density function),
we say the random variables are drawn \emph{iid}: independent and identically-distributed.
We stress that \emph{mutual} independence is a stronger restriction than
\emph{pairwise} independence: $m$ events $\{ E_i \}_{i=1}^m$ are mutually independent if
$\probability[\cap_i E_i] = \prod_i \probability[E_i]$.

We typically assume that data and query points are drawn \emph{iid} from some
(unknown) distribution. This is a standard and often necessary assumption
that eases analysis.

\section{Expectation and Variance}

The \emph{expected value} of a discrete random variable $X$ is denoted by $\ev[X]$
and defined as follows:
\begin{equation*}
    \ev[X] = \sum_x x \probability[X = x].
\end{equation*}
When $X$ is continuous, its expected value is based on the following Lebesgue integral:
\begin{equation*}
    \ev[X] = \int_{\Omega} X d \probability.
\end{equation*}
So when a random variable has probability density function $f_X$, its expected value
becomes:
\begin{equation*}
    \ev[X] = \int x f_X(x) dx.
\end{equation*}

For a \emph{nonnegative} random variable $X$, it is sometimes more convenient to
unpack $\ev{X}$ as follows instead:
\begin{equation*}
    \ev[X] = \int_0^\infty \probability[X > x] dx.
\end{equation*}

A fundamental property of expectation is that it is a linear operator.
Formally, $\ev[X + Y] = \ev[X] + \ev[Y]$ for two random variables $X$ and $Y$.
We use this property often in proofs.

We state another important property for independent random variables
that is easy to prove.
If $X$ and $Y$ are independent, then $\ev[XY] = \ev[X]\ev[Y]$.

\bigskip

The \emph{variance} of a random variable is defined as follows:
\begin{equation*}
    \var[X] = \ev\Big[ (X - \ev[X])^2 \Big] = \ev[X]^2 - \ev[X^2].
\end{equation*}
Unlike expectation, variance is not linear unless the random variables involved
are independent. It is also easy to see that $\var[aX] = a^2 \var[X]$ for a
constant $a$.

\section{Central Limit Theorem}
The result known as the Central Limit Theorem is one of the most
useful tools in probability. Informally, it states that the average of \emph{iid}
random variables with finite mean and variance converges to a Gaussian distribution.
There are several variants of this result that extend the claim to, for example,
independent but not identically distributed variables. Below we repeat the formal
result for the \emph{iid} case.

\begin{theorem}
    Let $X_i$'s be a sequence of $n$ \emph{iid} random variables with finite mean $\mu$
    and variance $\sigma^2$. Then, for any $x \in \mathbb{R}$:
    \begin{equation*}
        \lim_{n \rightarrow \infty} \probability \Big[
            \underbrace{\frac{(1/n \sum_{i=1}^n X_i) - \mu}{\sigma^2/n}}_Z \leq x
        \Big] = \int_{-\infty}^x \frac{1}{\sqrt{2 \pi}} e^{-\frac{t^2}{2}} dt,
    \end{equation*}
    implying that $Z \sim \mathcal{N}(0, 1)$.
\end{theorem}

\chapter{Concentration of Measure}
\label{appendix:measure}

\abstract{
By the strong law of large numbers, we know that the average of a sequence
of $m$ \emph{iid} random variables with mean $\mu$ converges to $\mu$ with
probability $1$ as $m$ tends to infinity. But how far is that average from
$\mu$ when $m$ is finite? Concentration inequalities helps us answer that question
quantitatively. This appendix reviews important inequalities that are used
in the proofs and arguments throughout this monograph.
}

\section{Markov's Inequality}

\begin{lemma}
    \label{lemma:appendix:concentration:markov}
    For a nonnegative random variable $X$ and a nonnegative constant $a \geq 0$:
    \begin{equation*}
        \probability[X \geq a] \leq \frac{\ev[X]}{a}.
    \end{equation*}
\end{lemma}
\begin{proof}
    Recall that the expectation of a nonnegative random variable $X$ can be written
    as:
    \begin{equation*}
        \ev[X] = \int_0^\infty \probability[X \geq x] dx.
    \end{equation*}
    Because $\probability[X \geq x]$ is monotonically nonincreasing, we can expand
    the above as follows to complete the proof:
    \begin{equation*}
        \ev[X] \geq \int_0^a \probability[X \geq x] dx \geq \int_0^a \probability[X \geq a] dx = a \probability[X \geq a].
    \end{equation*}
\end{proof}

\section{Chebyshev's Inequality}

\begin{lemma}
    \label{lemma:appendix:concentration:chebyshev}
    For a random variable $X$ and a constant $a > 0$:
    \begin{equation*}
        \probability \Big[ \big\lvert X - \ev[X] \big\rvert \geq a \Big] \leq \frac{\var[X]}{a^2}.
    \end{equation*}
\end{lemma}
\begin{proof}
    \begin{equation*}
        \probability \Big[ \big\lvert X - \ev[X] \big\rvert \geq a \Big] =
        \probability \Big[ \big( X - \ev[X] \big)^2 \geq a^2 \Big] \leq \frac{\var[X]}{a^2},
    \end{equation*}
    where the last step follows by the application of Markov's inequality.
\end{proof}

\begin{lemma}
    Let $\{ X_i \}_{i=1}^n$ be a sequence of iid random variables
    with mean $\mu < \infty$ and variance $\sigma^2 < \infty$. For $\delta \in (0, 1)$,
    with probability $1 - \delta$:
    \begin{equation*}
        \Big\lvert \frac{1}{n} \sum_{i = 1}^n X_i - \mu \Big\rvert \leq \sqrt{\frac{\sigma^2}{\delta n}}.
    \end{equation*}
\end{lemma}
\begin{proof}
    By Lemma~\ref{lemma:appendix:concentration:chebyshev}, for any $a > 0$:
    \begin{equation*}
        \probability \Bigg[ \Big\lvert \frac{1}{n}\sum_{i=1}^n X_i - \mu \Big\rvert \geq a \Bigg]
        \leq \frac{\sigma^2/n}{a^2}.
    \end{equation*}
    Setting the right-hand-side to $\delta$, we obtain:
    \begin{equation*}
        \frac{\sigma^2}{n a^2} = \delta \implies a = \sqrt{\frac{\sigma^2}{\delta n}},
    \end{equation*}
    which completes the proof.
\end{proof}

\section{Chernoff Bounds}

\begin{lemma}
    Let $\{ X_i \}_{i=1}^n$ be independent Bernoulli variables with success probability $p_i$.
    Define $X = \sum_i X_i$ and $\mu = \ev[X] = \sum_i p_i$. Then:
    \begin{equation*}
        \probability \Big[ X > (1 + \delta) \mu \Big] \leq e^{-h(\delta) \mu},
    \end{equation*}
    where,
    \begin{equation*}
        h(t) = (1 + t) \log(1 + t) - t.
    \end{equation*}
\end{lemma}
\begin{proof}
    Using Markov's inequality of Lemma~\ref{lemma:appendix:concentration:markov}
    we can write the following for any $t > 0$:
    \begin{equation*}
        \probability\Big[ X > (1 + \delta)\mu \Big] =
            \probability\Big[ e^{tX} > e^{t(1 + \delta)\mu} \Big] \leq
            \frac{\ev\big[ e^{tX} \big]}{e^{t (1 + \delta) \mu}}.
    \end{equation*}
    Expanding the expectation, we obtain:
    \begin{align*}
        \ev\big[e^{tX}\big] &= \ev\Big[ e^{t \sum_i X_i} \Big] = \ev\Big[ \prod_i e^{tX_i} \Big]
        = \prod_i \ev[e^{tX_i}] \\
        &= \prod_i \Big( p_i e^t + (1 - p_i) \Big) \\
        &= \prod_i \big( 1 + p_i (e^t - 1) \big) \\
        &\leq \prod_i e^{p_i(e^t - 1)} = e^{(e^t - 1)\mu}. && \text{by $(1 + t \leq e^t)$} \\
    \end{align*}
    Putting all this together gives us:
    \begin{equation}
        \label{equation:appendix:concentration:chernoff:proof}
        \probability\Big[ X > (1 + \delta)\mu \Big] \leq 
        \frac{e^{(e^t - 1) \mu}}{e^{t (1 + \delta) \mu}}.
    \end{equation}
    This bound holds for any value $t > 0$, and in particular a value of $t$ that
    minimizes the right-hand-side. To find such a $t$, we may differentiate
    the right-hand-side, set it to $0$, and solve for $t$ to obtain:
    \begin{align*}
        \frac{\mu e^t e^{(e^t - 1) \mu}}{e^{t (1 + \delta) \mu}} &-
        \mu ( 1 + \delta ) \frac{e^{(e^t - 1) \mu}}{e^{t (1 + \delta) \mu}} = 0 \\
        &\implies \mu e^t = \mu (1 + \delta) \\
        &\implies t = \log(1 + \delta).
    \end{align*}
    Substituting $t$ into Equation~(\ref{equation:appendix:concentration:chernoff:proof})
    gives the desired result.
\end{proof}

\section{Hoeffding's Inequality}

We need the following result, known as Hoeffding's Lemma, to present
Hoeffding's inequality.

\begin{lemma}
    \label{lemma:appendix:concentration:hoeffding-lemma}
    Let $X$ be a zero-mean random variable that takes values in $[a, b]$.
    For any $t > 0$:
    \begin{equation*}
        \ev\big[ e^{tX} \big] \leq \exp\Big( \frac{t^2 (b - a)^2}{8} \Big).
    \end{equation*}
\end{lemma}
\begin{proof}
    By convexity of $e^{tx}$ and given $x \in [a, b]$ we have that:
    \begin{equation*}
        e^{tx} \leq \frac{b - x}{b - a} e^{ta} +
            \frac{x - a}{b - a} e^{tb}.
    \end{equation*}
    Taking the expectation of both sides, we arrive at:
    \begin{equation*}
        \ev\Big[e^{tx}\Big] \leq
            \frac{b}{b - a} e^{ta} - \frac{a}{b - a} e^{tb}.
    \end{equation*}
    To conclude the proof, we first write the right-hand-side as
    $\exp(h(t(b - a)))$ where:
    \begin{equation*}
        h(x) = \frac{a}{b - a} x + \log \Big( \frac{b}{b - a} - \frac{a}{b - a} e^x \Big).
    \end{equation*}
    By expanding $h(x)$ using Taylor's theorem, it can be shown that
    $h(x) \leq x^2/8$. That completes the proof.
\end{proof}

We are ready to present Hoeffding's inequality.

\begin{lemma}
    Let $\{ X_i \}_{i=1}^n$ be a sequence of iid random variables
    with finite mean $\mu$ and suppose $X_i \in [a, b]$ almost surely.
    For all $\epsilon > 0$:
    \begin{equation*}
        \probability\Bigg[ \Big\lvert \frac{1}{n} \sum_{i=1}^n X_i - \mu \Big\rvert > \epsilon \Bigg] \leq 2 \exp\Big({-\frac{2n \epsilon^2}{(b - a)^2}}\Big).
    \end{equation*}
\end{lemma}
\begin{proof}
    Let $X = 1/n \sum_i X_i - \mu$. Observe by Markov's inequality that:
    \begin{equation*}
        \probability[X \geq \epsilon] = \probability\Big[ e^{tX} \geq e^{t\epsilon} \Big]
        \leq e^{-t\epsilon} \ev[e^{tX}].
    \end{equation*}
    By independence of $X_i$'s and
    the application of Lemma~\ref{lemma:appendix:concentration:hoeffding-lemma}:
    \begin{align*}
        \ev[e^{tX}] &= \ev \Bigg[ \prod_i e^\frac{t(X_i - \mu)}{n} \Bigg] \\
        &= \prod_i \ev \Big[ e^{\frac{t(X_i-\mu)}{n}} \Big] \\
        &\leq \prod_i \exp\Big( \frac{t^2 (b - a)^2}{8 n^2} \Big) \\
        &= \exp\Big( \frac{t^2 (b - a)^2}{8 n} \Big).
    \end{align*}
    We have shown that:
    \begin{equation*}
        \probability[X \geq \epsilon] \leq \exp\Big( -t \epsilon + \frac{t^2 (b - a)^2}{8 n} \Big).
    \end{equation*}
    That statement holds for all values of $t$ and in particular one that minimizes
    the right-hand-side. Solving for that value of $t$ gives us
    $t = 4n\epsilon / (b - a^2)$, which implies:
    \begin{equation*}
        \probability[X \geq \epsilon] \leq e^{-\frac{2n \epsilon^2}{(b - a)^2}}.
    \end{equation*}
    By a symmetric argument we can bound $\probability[X \leq -\epsilon]$. The claim
    follows by the union bound over the two cases.
\end{proof}

\section{Bennet's Inequality}

\begin{lemma}
    Let $\{ X_i \}_{i=1}^n$ be a sequence of independent random variables with zero mean
    and finite variance $\sigma_i^2$. Assume that $\lvert X_i \rvert \leq a$ almost surely for all $i$. Then:
    \begin{equation*}
        \probability\Big[\sum_i X_i \geq t \Big] \leq 
        \exp \Bigg( -\frac{\sigma^2}{a^2} h\Big( \frac{a t}{\sigma^2} \Big) \Bigg),
    \end{equation*}
    where $h(x) = (1 + x) \log(1 + x) - x$ and $\sigma^2 = \sum_i \sigma_i^2$.
\end{lemma}
\begin{proof}
    As usual, we take advantage of Markov's inequality to write:
    \begin{align*}
        \probability\Big[\sum_i X_i \geq t \Big] &\leq
            e^{-\lambda t} \ev \Big[ e^{\lambda \sum_i X_i} \Big] \\
        &= e^{-\lambda t} \ev \Big[ \prod_i e^{\lambda X_i} \Big] \\
        &= e^{-\lambda t} \prod_i \ev \Big[ e^{\lambda X_i} \Big] \\
    \end{align*}
    Using the Taylor expansion of $e^x$, we obtain:
    \begin{align*}
        \ev \Big[ e^{\lambda X_i} \Big] &= \ev \Big[ \sum_{k=0}^\infty \frac{\lambda^k X_i^k}{k!} \Big] \\
        &= 1 + \sum_{k=2}^\infty \frac{\lambda^k \ev[X_i^2 X_i^{k - 2}]}{k!} \\
        &\leq 1 + \sum_{k=2}^\infty \frac{\lambda^k \sigma_i^2 a^{k-2}}{k!} \\
        &= 1 + \frac{\sigma_i^2}{a^2} \sum_{k=2}^\infty \frac{\lambda^k a^k}{k!} \\
        &= 1 + \frac{\sigma_i^2}{a^2} \big( e^{\lambda a} - 1 - \lambda a \big) \\
        &\leq \exp\Big( \frac{\sigma_i^2}{a^2} \big( e^{\lambda a} - 1 - \lambda a \big) \Big).
    \end{align*}
    Putting it all together:
    \begin{align*}
        \probability\Big[\sum_i X_i \geq t \Big] &\leq
            e^{-\lambda t} \prod_i \exp\Big( \frac{\sigma_i^2}{a^2} \big( e^{\lambda a} - 1 - \lambda a \big) \Big) \\
        &= e^{-\lambda t} \exp\Big( \frac{\sigma^2}{a^2} \big( e^{\lambda a} - 1 - \lambda a \big) \Big).
    \end{align*}
    This inequality holds for all values of $\lambda$, and in particular one that minimizes the
    right-hand-side. Setting the derivative of the right-hand-side to $0$ and solving for $\lambda$
    leads to the desired result.
\end{proof}

\chapter{Linear Algebra Review}
\label{appendix:linear-algebra}

\abstract{
This appendix reviews basic concepts from Linear Algebra that are useful
in digesting the material in this monograph.
}

\section{Inner Product}

Denote by $\mathbb{H}$ a vector space.
An inner product $\langle \cdot, \cdot \rangle: \mathbb{H} \times \mathbb{H} \rightarrow \mathbb{R}$
is a function with the following properties:
\begin{itemize}
    \item $\forall \; u \in \mathbb{H},\; \langle u, u \rangle \geq 0$;
    \item $\forall \; u \in \mathbb{H},\; \langle u, u \rangle = 0 \Leftrightarrow u = 0$;
    \item $\forall \; u, v \in \mathbb{H},\; \langle u, v \rangle = \langle v, u \rangle$; and,
    \item $\forall \; u, v, w \in \mathbb{H}, \textit{ and } \alpha, \beta \in \mathbb{R},\; 
    \langle \alpha u + \beta v, w \rangle = \alpha \langle u, w \rangle + \beta \langle v, w \rangle$.
\end{itemize}

We call $\mathbb{H}$ together with the inner product $\langle \cdot, \cdot \rangle$
an \emph{inner product space}.
As an example, when $\mathbb{H} = \mathbb{R}^d$, given two vectors
$u = \sum_{i=1}^d u_i e_i$ and $v = \sum_{i=1}^d v_i e_i$, where $e_i$'s
are the standard basis vectors, the following is an inner product:
\begin{equation*}
    \langle u, v \rangle = \sum_{i = 1}^d u_i v_i.
\end{equation*}

We say two vectors $u$ and $v$ in an inner product space are \emph{orthogonal}
if their inner product is $0$: $\langle u, v \rangle = 0$.

\section{Norms}

A function $\Phi: \mathbb{H} \rightarrow \mathbb{R}_+$ is a norm on
$\mathbb{H}$ if it has the following properties:
\begin{itemize}
    \item Definiteness: For all $u \in \mathbb{H}$, $\Phi(u) = 0 \Leftrightarrow u = 0$;
    \item Homogeneity: For all $u \in \mathbb{H}$ and $\alpha \in \mathbb{R}$,
        $\Phi(\alpha u) = \lvert \alpha \rvert \Phi(u)$; and,
    \item Triangle inequality: $\forall \; u, v \in \mathbb{H}, \; \Phi(u + v) \leq \Phi(u) + \Phi(v)$.
\end{itemize}

Examples include the absolute value on $\mathbb{R}$,
and the $L_p$ norm (for $p \geq 1$) on $\mathbb{R}^d$ denoted by $\lVert \cdot \rVert_p$
and defined as:
\begin{equation*}
    \lVert u \rVert_p = \Big( \sum_{i=1}^d \lvert u_i \rvert^p \Big)^{\frac{1}{p}}.
\end{equation*}
Instances of $L_p$ include the commonly used $L_1$, $L_2$ (Euclidean),
and $L_\infty$ norms, where $\lVert u \rVert_\infty = \max_i \lvert u_i \rvert$.

Note that, when $\mathbb{H}$ is an inner product space, then
the function $\lVert u \rVert = \sqrt{\langle u, u \rangle}$ is a norm.

\section{Distance}
A norm on a vector space induces a notion of distance between two vectors.
Concretely, if $\mathbb{H}$ is a normed space equipped with $\lVert \cdot \rVert$,
then we define the distance between two vectors $u, v \in \mathbb{H}$ as follows:
\begin{equation*}
    \delta(u, v) = \lVert u - v \rVert.
\end{equation*}

\section{Orthogonal Projection}

\begin{lemma}
    Let $\mathbb{H}$ be an inner product space and suppose $u \in \mathbb{H}$ and $u \neq 0$.
    Any vector $v \in \mathbb{H}$ can be uniquely decomposed along $u$ as:
    \begin{equation*}
        v = v_{\perp} + v_{\parallel},
    \end{equation*}
    such that $\langle v_\perp, v_\parallel \rangle = 0$. Additionally:
    \begin{equation*}
        v_\parallel = \frac{\langle u, v \rangle}{\langle u, u \rangle} u,
    \end{equation*}
    and $v_\perp = v - v_\parallel$.
\end{lemma}
\begin{proof}
    Let $v_\parallel = \alpha u$ and $v_\perp = v - v_\parallel$.
    Because $v_\parallel$ and $v_\perp$ are orthogonal, we deduce that:
    \begin{align*}
        \langle v_\parallel, v_\perp \rangle = 0 \implies
            \langle \alpha u, v_\perp \rangle = 0 \implies
            \langle u, v_\perp \rangle = 0.
    \end{align*}
    That implies:
    \begin{align*}
        \langle v, u \rangle = \alpha \langle u, u \rangle \implies
        \alpha = \frac{\langle u, v \rangle}{\langle u, u \rangle},
    \end{align*}
    so that:
    \begin{equation*}
        v_\parallel = \frac{\langle u, v \rangle}{\langle u, u \rangle} u.
    \end{equation*}

    We prove the uniqueness of the decomposition by contradiction.
    Suppose there exists another decomposition of $v$ to $v_\parallel^\prime + v_\perp^\prime$.
    Then:
    \begin{align*}
        v_\parallel + v_\perp = v_\parallel^\prime + v_\perp^\prime &\implies
        \langle u, v_\parallel + v_\perp \rangle = \langle u,  v_\parallel^\prime + v_\perp^\prime\rangle \\
        &\implies \langle u, v_\parallel \rangle = \langle u,  v_\parallel^\prime \rangle \\
        &\implies \langle u, \alpha u \rangle = \langle u, \beta u \rangle \\
        &\implies \alpha = \beta.
    \end{align*}
    We must therefore also have that $v_\perp = v_\perp^\prime$.
\end{proof}
